# Supplementary material for: On the Convergence Rate of Off-Policy Policy Optimization Methods with Density-Ratio Correction
Source: arXiv:2106.00993 source file (2022-02-13)
Supplement: Supplementary file 1 [file Appendix_Compare2Oracles.tex]

\section{A Comparison between Two Oracle Examples}\label{appx:compare2Oracles}
In this section, we will make a comparison between two Oracle Algorithms: Alg \ref{alg:PLSO} and Alg \ref{alg:SVREB} about the computational complexity and solution quality. We compare the upper bounds of two Algorithms for the value $\sqrt{\EE[\|\hat\zeta-\zeta^*\|^2+\|\hat\xi-\xi^*\|^2]}$ after consuming $N$ samples.

For simplification, we fix $Z=\{\zeta|\|\zeta\|\leq \rad_\zeta\}$ and $\Xi=\{\xi|\|\xi\|\leq \rad_\xi\}$, where $\rad_\zeta$ and $\rad_\xi$ are defined in \ref{def:Rzeta} and \ref{def:Rxi}. 
Besides, we focus on the case when $N>> d, \sigma_\K, \sigma_\M, \sigma_\nu, \sigma_R$, $\lambda_w= \lambda_Q =\lambda\leq 1$, $\dims_\zeta=\dims_\xi=d$ and $\eig_w=\eig_Q=\eig_{\min}$. Now we start our comparison.

\paragraph{The quality of the solution returned by Least-Square oracle}
Recall the results we obtained in Eq.\eqref{eq:exp_quality_dm},
\begin{align*}
    &\sqrt{\EE[\|\zeta^*-\hat\zeta^*\|^2+\|\xi^*-\hat\xi^*\|^2]}\\
    =&O\Big(\frac{1+\lambda_Q\eig_Q}{\eig_Q (\lambda_w\lambda_Q\eig_w+\eig_\M^2)^2\sqrt{N_{all}}}(\lambda_w\lambda_Q \sigma_\K + \frac{\sigma_\M}{\eig_Q}+\frac{\sigma_\K}{\eig^2_Q})+\frac{\sigma_\nu}{\eig_Q(\lambda_w\lambda_Q \eig_w + \eig_\M^2)\sqrt{N_{all}}}+\frac{\lambda_Q\sigma_R}{(\lambda_w\lambda_Q \eig_w + \eig_\M^2)\sqrt{N_{all}}}\\
    &+\frac{\lambda_w\eig_w+1}{\eig_w(\lambda_w\lambda_Q\eig_Q+\eig_\M)^2\sqrt{N_{all}}}(\lambda_w\lambda_Q \sigma_\K + \frac{\sigma_\M}{\eig_w}+\frac{\sigma_\K}{\eig_w^2})+\frac{\sigma_R}{\eig_w(\lambda_w\lambda_Q \eig_Q + \eig_\M^2)\sqrt{N_{all}}}+\frac{\lambda_w\sigma_\nu}{(\lambda_w\lambda_Q \eig_Q + \eig_\M^2)\sqrt{N_{all}}}\Big)\\
    =&O\Big(\frac{(1+\lambda\eig_{\min})(\lambda^2\eig_{\min}^2\sigma_\K+\eig_{\min}\sigma_\M + \sigma_\K)}{\eig_{\min}^3(\lambda^2\eig_{\min}+\eig_\M^2)^2\sqrt{N_{all}}}+\frac{(\lambda\eig_{\min}+1)(\sigma_\nu+\sigma_R)}{\eig_{\min}(\lambda^2 \eig_{\min} + \eig_\M^2)\sqrt{N_{all}}}\Big)\sqrt{d}
\end{align*}

\paragraph{The quality of the solution returned by SVRE}

% In SVRE, to make sure $\EE[\|\zeta^* - \hat{\zeta}^*\|^2 + \|\xi^* - \hat{\xi}^*\|^2]\leq \epsilon^2$, we may choose to iterate $O(\log \frac{1}{\epsilon})$ loops with batch size $O(\frac{1}{\epsilon^2})$, which results in the total number of samples are $O(\epsilon^{-2})$. Combining the analysis for the direct solution above, we know that with high probability, $\|\zeta^* - \hat{\zeta}^*\|^2 + \|\xi^* - \hat{\xi}^*\|^2=O(\epsilon^2)$. As a conclusion, both two methods has a similar performance. The direct method has a stronger guarantee with high probability while SVRE only guarantee the expected performance (but we can use \Markov's inequality to obtain a relatively high probability bound). However, as for the computational complexity, SVRE enjoy $O(\frac{n}{\epsilon^{2}})$ while the direct method is at least $O((\frac{n}{\epsilon})^2)$, which means SVRE is quite efficient, especially when the dimension of features are very large.

In SVRE, in order to make sure $\EE[\|\zeta_\K-\zeta^*\|^2+\|\xi_\K-\xi^*\|^2]\leq \epsilon^2$, we may choose to iterate $k$ times with batch size $b$ satisfying:
\begin{align*}
    (1-\min\{\frac{\mz\ez}{4},\frac{\mx\ex}{4}\})^k  \leq \frac{\epsilon^2}{8\rad_\zeta^2 + 8\rad_\xi^2}\\
    \frac{8\sigma^2}{\min\{\frac{\mz\ez}{4},\frac{\mx\ex}{4}\}b}(\frac{\ez}{\mz}+\frac{\ex}{\mx})\leq \frac{\epsilon^2}{2}
\end{align*}

In the proof of Condition \ref{cond:variance}, we have proved that:
\begin{align*}
    \EE_{s,a,r,s',a_0,a'}[\|\nz \cL^{(s,a,r,s',a_0,a')}(\theta,\zeta,\xi)-\nz \cL^D(\theta,\zeta,\xi)\|^2]=& O(\sigma_R^2 + \sigma^2_\M \rad_\xi^2 + \lambda^2_w\sigma_\K^2 \rad_\zeta^2)\\
    \EE_{s,a,r,s',a_0,a'}[\|\nx \cL^{(s,a,r,s',a_0,a')}(\theta,\zeta,\xi)-\nx \cL^D(\theta,\zeta,\xi)\|^2]=& O(\sigma^2_{\nu}+\sigma^2_\M \rad_\zeta^2 + \lambda^2_Q\sigma^2_\K \rad_\xi^2)
\end{align*}
which implies
\begin{align*}
    \sigma^2 \approx& \sigma_\nu^2 + \sigma^2_R + \sigma^2_\M (\rad_\zeta^2 + \rad_\xi^2)+ \sigma_\K^2(\lambda^2_w\rad
    _\zeta^2+\lambda^2_Q \rad_\xi^2)\\
    =&\sigma_\nu^2 + \sigma^2_R + (\sigma^2_\M +\lambda^2 \sigma_\K^2)(\rad_\zeta^2 + \rad_\xi^2)
\end{align*}
Besides, we have,
\begin{align*}
    \mz =\mx=\lambda\eig_{\min},~~~\ez=\ex=\frac{1}{50\bar{L}},~~~\bar{L}=\frac{2\max\{\lambda^2_w, \lambda^w_Q\} + 2(1+\gamma)^2}{\min\{\lambda_w\eig_w, \lambda_Q\eig_Q\}}=O(\frac{1}{\lambda \eig_{\min}})\\
\end{align*}
% \frac{1-\gamma}{\eig_{\min}} + \frac{\lambda}{\lambda^2 \eig+ \sigma^2_{\min}}
% \frac{(1-\gamma)\lambda}{\lambda^2 \eig+\sigma^2_{\min}}+\frac{1}{\eig_{\min}}
which implies that
\begin{align*}
    k \geq &\log \frac{\epsilon^2}{8\rad_\zeta^2 +8\rad_\xi^2}\log^{-1} (1-\min\{\frac{\mz\ez}{4},\frac{\mx\ex}{4}\}) = O(\frac{1}{\lambda^2{\eig_{\min}^2}})\\
    b\geq& \frac{16\sigma^2}{\min\{\frac{\mz\ez}{4},\frac{\mx\ex}{4}\}\epsilon^2}(\frac{\ez}{\mz}+\frac{\ex}{\mx})=O(\frac{\sigma_\nu^2 + \sigma^2_R + (\sigma^2_\M + \lambda^2\sigma_\K^2)(\rad_\zeta^2 + \rad_\xi^2)}{\lambda^2{\eig_{\min}^2}\epsilon^2})
\end{align*}
The total number of samples denoted as $N_{all}'$ should be
\begin{align*}
    N_{all}'=k\cdot b=O(\frac{\sigma_\nu^2 + \sigma^2_R + (\sigma^2_\M + \lambda^2\sigma_\K^2)(\rad_\zeta^2 + \rad_\xi^2)}{\lambda^4\eig_{\min}^4\epsilon^2})
\end{align*}
In another word,
\begin{align*}
    &\sqrt{\EE[\|\hat\zeta-\zeta^*\|^2+\|\hat\xi-\xi^*\|^2]} \\
    =& O(\frac{1}{\lambda^2{\eig_{\min}^2}\sqrt{N_{all}'}}\sqrt{\sigma_\nu^2 + \sigma_R^2+(\sigma^2_\M+\lambda^2\sigma^2_\K)(\rad_\zeta^2 + \rad_\xi^2)})\\
    =& O(\frac{1}{\lambda^2{\eig_{\min}^2}\sqrt{N_{all}'}}\Big(\sigma_\nu + \sigma_R+(\sigma_\M+\lambda \sigma_\K) (\rad_\zeta + \rad_\xi) \Big))\\
    =& O(\frac{1}{\lambda^2{\eig_{\min}^2}\sqrt{N_{all}'}}\Big(\sigma_\nu + \sigma_R+ \frac{(\lambda\eig_{\min}+1)(\sigma_\M+\lambda \sigma_\K)}{\eig_{\min}(\lambda^2\eig_{\min} + \eig^2_\M)} \Big))\numberthis\label{eq:quality_svre}
\end{align*}

% \subsection{Related Work}
% As for previous works considering off-policy evaluation with linear function classes, in \citep{}, the authors used a saddle-point formulation which can be regarded as a special case of ours after dropping the regularization on $Q$. They also pointed out the connection with the GTD family algorithms and. However, they have a worse dependence on $N$ than ours because of the lack of regularization on parameters of $Q$ function.

\subsection{Comparison between two Oracles}
\paragraph{Dependence on the number of samples ($N_{all}$ and $N_{all}'$)} Easy to observe that, both of them have the same dependence on the number of samples. 
\paragraph{Dependence on $\eig_{\min}$ and $\eig_\M$} Because we already assume that $\|\bphi(\cdot, \cdot)\|\leq 1$, we have $tr(\K)\leq 1$, which implies that $\eig_{\min}\leq \frac{1}{d}$. Therefore, the dependence of $\frac{1}{\eig_{\min}}$ in some degree reflects the dependence on $d$ and can also take a great effect on efficiency when $d$ is very large. As we can see that, if we fix other parameters, the worst dependence of the SVRE oracle is $\eig_{\min}^{-3}(\eig_{\min}+\eig_\M^2)^{-1}$, which is slightly better than $\eig_{\min}^{-3}(\eig_{\min}+\eig_\M^2)^{-2}$ of the least-square oracle. Besides, the least-square oracle has an additional dependence on $\sqrt{d}$.

\paragraph{Dependence on $\lambda$} 
As we can see, the quality of SVRE's solution depends on $\lambda^{-2}$. In constrat, the direct method is much more stable, and has a lower bound as $\lambda$ approaching 0. 
It's a reasonable result, because SVRE is a first-order optimization algorithm and its convergence rate depends on the condition number of the problem, while in the least-square method we can directly solve the saddle-point and inaccuracy only comes from the randomness of $\hK$, $\hM$ and etc.

\paragraph{Dependence on variance terms} We can see they have the same dependence on $\sigma_\K, \sigma_\M, \sigma_\nu$ and $\sigma_R$.

\paragraph{Computational Complexity} In direct methods it costs $O(d^2)$ operation for one sample, and the matrix inverse will consume $O(d^3)$. Since we consider the case when $N>>d$ and therefore it's $O(Nd^2)$ in total. As for SVRE, we only need $O(d)$ for each sample and the total complexity is $O(Nd)$, which has less dependence on $d$.

As a conclusion, when we choose small $\lambda$, the least-square oracle is faster and also preferable if we donot mind computational complexity. Otherwise, we may want to use SVRE, because its convergence rate has a better dependence on the sigular values and the computation is efficiency. Moreover, least-sqaure oracle can only be used in linear setting, while SVRE can be extended to other strongly-convex-strongly-concave setting.
